# Supplementary material for: On the sensitivity of the simulated European Neolithic transition to climate extremes
Source: arXiv:1203.0222 source file (2012-08-11)
Supplement: Supplementary file 1 [file supplementary_material.pdf]

# Supplementary material for “On the sensitivity of the simulated European Neolithic transition to climate extremes”

Carsten Lemmen\*, Kai W. Wirtz

*Helmholtz-Zentrum Geesthacht, Institut für Küstenforschung, Max-Planck Straße 1, 21501 Geesthacht, Germany*

## 1. Supplementary information on GLUES

The Global Land Use and technological Evolution Simulator (GLUES, [Wirtz and Lemmen, 2003](#); [Lemmen, 2010](#); [Lemmen and Wirtz, 2010](#)) mathematically resolves the dynamics of human populations and their characteristic sociocultural traits in the context of a changing biogeographical environment. A local sociocultural coevolution is described by changes in mean population density (P), technology (T), share of agropastoral activities (Q), and economic diversity (N), within a simulation region of approximately country-size extent (Figure 1 of main manuscript). Each region’s population utilises its natural resources, which are described by environmental utility (FEP) and climate constraints (TLI). While the mathematical implementation is summarised in its entirety from [Wirtz and Lemmen \(2003\)](#), the reader is advised to refer to the original manuscript for detailed motivation for each model assumption.

### 1.1. Characteristic trait dynamics

For pre-industrial human societies, [Wirtz and Lemmen \(2003\)](#) defined three characteristic traits  $X \in \{T, Q, N\}$ :

1. Technology (T) is a trait which describes the efficiency of food procurement related to both foraging and farming.
2. A second model variable (Q) describes the allocation of energy, time, or manpower to agropastoralism.
3. Economic diversity (N), resolves the number of different economies in the agropastoral sector which are available to a region’s population.

The evolution of each of these traits (X) follows the direction of increased benefit for success (i.e., growth benefit  $\partial r / \partial X$ ) of its associated population; this concept had been derived for genetic traits in the works of [Fisher \(1930\)](#), and more recently by Metz and colleagues (e.g. [Kisdi and Geritz, 2010](#)) as adaptive dynamics (AD). In AD, the population averaged value of a trait changes at a rate which is proportional to the gradient of the fitness function, evaluated the mean trait value:

$$\frac{dX}{dt} = \delta_X \frac{\partial r}{\partial X} \quad X \in \{T, Q, N\}, \quad (1)$$

where  $\delta_X$  is the so-called flexibility for trait X and is often given by the variance of X;  $r$  denotes the relative growth rate of the population, i.e.  $r = (dP/dt)/P$ .

### 1.2. Productivity and growth

The Neolithic transition is characterised by changes in subsistence intensity (SI). Subsistence intensity describes a community’s effectiveness in generating consumable food and secondary products; this can be achieved based on an agricultural (with fractional activity Q) and a hunting-gathering life style (with fractional activity  $1 - Q$ ). SI is dimensionless and scaled such that a value of unity expresses the mean subsistence intensity of a hunter-gatherer society equipped with tools typical for the mature Mesolithic and living in an affluent natural environment.

$$SI = (1 - Q) \cdot \sqrt{T} + Q \cdot N \cdot T \cdot TLI \quad (2)$$

The agricultural part of SI increases linearly with N and with T: The more economies (N) there are, the better are sub-regional scaled niches utilised and the more reliable returns are generated when annual weather conditions are variable; the higher the technology level (T), the better the efficiency of using natural resources (by definition of T). While a variety of techniques can steeply increase harvests of domesticated species, analogous benefits for foraging productivity are less pronounced and justify a less than linear dependence of the hunting-gathering calorie procurement on T. We use a square root formulation, which satisfies  $\sqrt{T} < T$  since T is generally larger than unity.

We introduce an additional temperature constraint (TLI) on agricultural productivity which considers that cold temperature could only moderately be overcome by Neolithic technologies. This limitation is unity at low latitudes and approaches zero at permafrost conditions.

The domestication process is represented by N, which is the number of realised agropastoral economies. We link N to natural resources by expressing it as the fraction  $f$  of potentially available economies (PAE) by specifying  $N = f \cdot PAE$ , where the latter corresponds to the richness in domesticable animal or plant species within a specific region.

### 1.3. Food productivity and human growth rate

The growth rate  $r$  of a regional population relative to its size is mainly controlled by its subsistence intensity SI:

\*Tel +49 4152 87-2013, Fax -2020

Email address: [carsten.lemmen@hzg.de](mailto:carsten.lemmen@hzg.de) (Carsten Lemmen)

$$r = \mu \cdot (\text{FEP} - \gamma\sqrt{\text{TP}}) \cdot (1 - \omega T) \cdot \text{SI} - \rho \cdot P \cdot e^{-T/T_{\text{lit}}}, \quad (3)$$

with growth rate parameters  $\mu$  and  $\rho$ . The subsistence intensity's contribution to growth is modulated by environmental utility (FEP), societal impacts on the environment ( $-\gamma\sqrt{\text{TP}}$ ), and organisational losses within a society ( $1 - \omega T$ ). As technology advances, more and more people neither farm nor hunt: Construction, maintenance, administration draw a small fraction  $\omega$  of the workforce away from food-production. The impact on the environment is modelled as a function of population density and technology (IPAT, [Ehrlich and Holdren, 1971](#)) on the utility of the environment (FEP, see next section). The loss term is mediated by technologies ( $T$ , with  $T_{\text{lit}} = 12$ ), which mitigate, for example, losses due to disease. The implementation of the loss term differs from the originally inverse formulation by [Wirtz and Lemmen \(2003,  \$-\rho \frac{P}{T}\$ \)](#), but is numerically simpler and phenologically similar.

#### 1.4. Region definition

GLUES operates on a set of regions which, in turn, are defined on a high resolution ( $0.5^\circ \times 0.5^\circ$ ) grid. The region definition is implemented as a Cellular Automaton (CA), and resembles the application of a spatial low-pass filter to the grid. The CA formalism facilitates a dynamisation of region boundaries in future model applications. The CA aims at describing the organisation of local Mesolithic and Neolithic populations as cultural complexes that share common traits across larger spatial scales. The algorithm combines single adjacent cells into a cluster (region), starting from a distribution where each cell forms an individual cluster. The CA iteratively computes the similarity in geographical characteristics between neighbour cells. Similarity is defined as the sum of absolute and normalised differences in discriminating local properties (NPP and growing degree days). The similarities to all neighbour cells are weighted by a factor  $A/(A + A_T)$  where  $A$  denotes the area of the adjacent cluster and  $A_T$  a predefined target cluster size. The neighbour cell with maximal area weighted similarity then inherits cluster membership to the original cell. Cells that together with similar neighbours already form a cluster, usually do not change membership, while cells with a regionally anomalous biogeography become part of a new cluster. As a result, larger clusters incorporate cells at their boundary in relation to their own size and biogeographical similarity. The cluster distribution reaches a steady state when most cells are organised in clusters of relatively large cell number ( $A > 2A_T$ ). Small clusters below the threshold size  $A_T$  may, however, persist depending on the topography and the choice of  $A_T$ ; these are attached to one of the adjacent cluster regions using the area weighted similarity computed at the cluster scale.

#### 1.5. Coupling to biogeography

We reconstruct past distributions of net primary production (NPP) using a global climate model coupled to

a vegetation module. From Climber-2 ([Claussen and Brovkin, 1999](#)) temperature ( $t$ ) and precipitation ( $p$ ) anomalies on the IIASA climatological database ([Leemans and Cramer, 1991](#)) we calculated NPP following [Lieth \(1975, Miami model\)](#):

$$\begin{aligned} \text{NPP}_p &= \left(1 - e^{-0.664p/\text{m}}\right) \cdot \frac{1460 \text{ g}}{\text{m}^2 \text{ a}} \\ \text{NPP}_t &= \left(1 + 3.7248 e^{-0.119t/^\circ\text{C}}\right)^{-1} \cdot \frac{1460 \text{ g}}{\text{m}^2 \text{ a}} \\ \text{NPP} &= \min(\text{NPP}_p, \text{NPP}_t) \end{aligned} \quad (4)$$

Local food extraction potential (FEP) represents the utility of a multidimensional environment for food production; this FEP generally increases with NPP; at very high (i.e. tropical) NPP, it decreases because the amount of non-usable biomass rises ([Bloom et al., 1998](#)) and the crop yield declines ([Gallup and Sachs, 2000](#)). We choose  $\text{NPP}_F = 1100 \text{ gm}^{-2} \text{ a}^{-1}$  to describe the productivity where FEP is highest and derive FEP as follows:

$$\text{FEP} = \frac{2 \frac{\text{NPP}}{\text{NPP}_F}}{\left(\frac{\text{NPP}}{\text{NPP}_F}\right)^2 + 1} \quad (5)$$

According to [Braidwood and Braidwood \(1949\)](#)'s hilly flanks hypothesis, potential domesticates were most abundant in open woodlands, which are characterised by low to moderate NPP; we accordingly use a monomodal transfer function to calculate the relative local potential for agropastoral economies (LAE), with a maximum at  $\text{NPP}_N = 550 \text{ gm}^{-2} \text{ a}^{-1}$ .

$$\text{LAE} = \text{TLI} \cdot \frac{4 \frac{\text{NPP}}{\text{NPP}_N}}{\left(\frac{\text{NPP}}{\text{NPP}_N}\right)^3 + 3} \quad (6)$$

Temperature limitation is included in the calculation of LAE because cold-adapted plants do generally not carry usable large seeds, fruits or tubers.

Following the concept of, for example, [Gaston \(2000\)](#) for the connection of species richness on two different spatial scales, we connect the relative local potential (LAE) with the continental potential for agropastoral economies (CAE) to obtain an absolute local potential for agriculture (PAE); this way, we also account for continental aggregation area-biodiversity relationships. Let  $i$  denote a region index and  $\mathcal{I}_k$  the set of regions on continent  $k$ . Then

$$\text{PAE}_i = \text{LAE}_i \cdot \text{CAE}_k \quad \text{for} \quad i \in \mathcal{I}_k \quad (7)$$

As continents, we consider seven ( $k \in \{1 \dots 7\}$ ) large biogeographic units: Australia, Sub-Saharan Africa, Eurasia including North Africa, North America, South America, Greenland, and one unit consisting of all large islands. To obtain  $\text{CAE}_k$ , we calculate a weighted sum of all LAE with region area  $A_i$  on continent  $k$ , and scale with the values for the largest continent (Eurasia) where  $\text{CAE}_k = \text{CAE}_{\text{max}}$  and  $A_k = A_{\text{max}}$ . The consideration of

region areas  $A_i$  represents a linearised species-area relationship (Begon et al., 1993).

$$\text{CAE}_k = \text{CAE}_{\max} \cdot A_{\max}^{-1} \cdot \sum_{i \in \mathcal{I}_k} (A_i \cdot \text{LAE}_i). \quad (8)$$

### 1.6. Interregional exchange

Exchange between region  $i$  and its neighbour  $j$  in the neighbourhood  $\mathcal{N}_i$  comprises communication, trade, colonisation, warfare, migration of individuals or entire populations. We use the concept of influence by Renfrew and Level (1979), defined by us as the product of P and T to reflect imbalances in population pressure and disparate technologies. Influence differences relative to the spatial average  $\langle T \cdot P \rangle_{ij}$  act as a driving force  $f_{ij}$  for exchange. The flux  $f_{ij}$  is formulated as a first order relaxation (e.g. Wang and van Cappellen, 1996) and depends on (1) the influence difference, (2) common boundary length  $L_{ij}$  of the two regions, (3) the distance of their centres  $\sqrt{A_i A_j}$ , and (4) exchange coefficients for spread with people  $\sigma_P$  and without  $\sigma_T$ .

$$f_{ij} = \sigma_{P,T} \frac{L_{ij}}{\sqrt{A_i A_j}} \cdot (\langle T \cdot P \rangle_{ij} - T_i P_i) \quad (9)$$

Whenever there is a positive flux  $f_{ij} > 0$ , trait value differences in traits T and N from its neighbourhood  $\mathcal{N}_i$  are added to region  $i$ 's traits:

$$\left. \frac{dX_i}{dt} \right|_T = \sum_{j \in \mathcal{N}_i, f_{ij} > 0} f_{ij} \cdot (X_j - X_i) \quad (10)$$

Population diffusion is mass-conserving and is composed of immigration ( $f_{ij} > 0$ ) and emigration ( $f_{ij} < 0$ ) of individuals or groups.

$$\left. \frac{dP_i}{dt} \right|_P = \sum_{j \in \mathcal{N}_i, f_{ij} > 0} f_{ij} P_j \frac{A_j}{A_i} - \sum_{j \in \mathcal{N}_i, f_{ij} < 0} f_{ij} P_i \quad (11)$$

With immigrating people, the characteristic traits of the migrants are carried over to the receiving region:

$$\left. \frac{dX_i}{dt} \right|_P = \sum_{j \in \mathcal{N}_i, f_{ij} > 0} f_{ij} X_j \frac{P_j A_j}{P_i A_i} \quad (12)$$

### 1.7. Cultural memory loss

When population declines, a cultural loss (loss of technology and applied economies) is imposed on a regional society. This loss is described by Lemmen (2010) and formulated as

$$\left. \frac{dX_i}{dt} \right|_{\text{crisis}} = \beta \cdot r \cdot X \quad (13)$$

Where  $\beta$  describes the percentage of knowledge loss at a given relative loss in population number. In this study, we set  $\beta = 0.8$

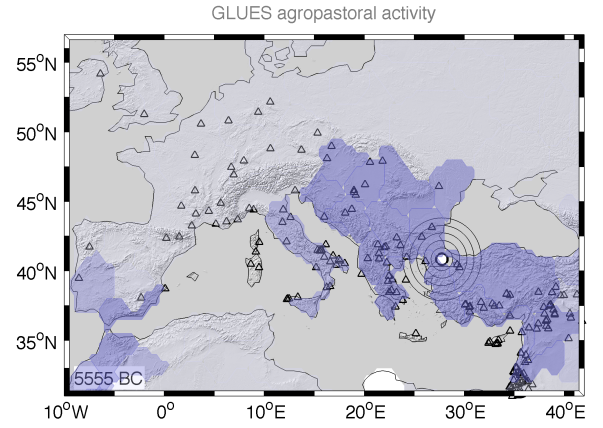

Figure 1: Expansion of farming activity across Europe. Snapshot of the movie supplied with this supplementary material. Blue shading indicates regions with predominant farming activity; triangles show the location of radiocarbon dated Neolithic archaeological sites; white dots show the location and duration of climate events diagnosed from globally 134 palaeoclimate records.

Table 1: Table of 134 palaeoclimate time series, of which 122 were analysed by Wirtz et al. (2010, their Table 2). Abbreviations: Lk=Lake, Cv=Cave, LG=lithic grains, SST=sea surface temperature, T=temperature, T7=July temperature, P=precipitation, GSD=grayscale density, HSG=hematite stained glass, SSS=sea surface salinity, Ef=effective, LG=lithic grains, Nitz.=Nitzschia, Ozean.=Ozeanica, Ti=Titanium content

| No | Site                | Proxy                      | Events (cal BC)        | Reference                      | No  | Site                     | Proxy                      | Events (cal BC)             | Reference                      |
|----|---------------------|----------------------------|------------------------|--------------------------------|-----|--------------------------|----------------------------|-----------------------------|--------------------------------|
| 1  | NW Alaska           | Mg/Ca T                    | 7370/6530              | Hu et al. 1998                 | 68  | N Finland                | T                          | 6940/5160                   | Husum and Hald 2004            |
| 2  | NW Pacific          | $\delta^{18}\text{O}$      | none                   | Oba and Murayama 2004          | 69  | N Atlantic               | GSD                        | 9380/9300<br>8090/3790      | Chapman and Shackleton 2000    |
| 3  | Owens Lk, CA        | $\delta^{18}\text{O}$      | 9180                   | Benson et al. 2002             | 70  | Marmara Sea              | $\delta^{18}\text{O}$      | 3590/3230                   | Sperling et al. 2003           |
| 4  | E California        | P                          | 6910/6390              | Hughes and Graulich 1996       | 71  | Marmara Sea              | $\text{U}_{37}^k$ SST      | 7640/7250/3500              | Sperling et al. 2003           |
| 5  | W Canada            | Density                    | 6950/6230/4680         | Yu 2003                        | 72  | SE Africa                | $\delta^{18}\text{O}$      | 9100                        | Holmgren et al. 2003           |
| 6  | S California        | Moisture                   | 5850                   | Davis 1992                     | 73  | Burundi                  | P                          | 9500/7320                   | Bonnefille and Chalié 2000     |
| 7  | Moon Lk, ND         | Salinity                   | none                   | Laird et al. 1996              | 74  | Black Sea                | Ti                         | 7220                        | Bahr et al. 2005               |
| 8  | Kimble, MN          | Charcoal                   | 3010                   | Camill et al. 2003             | 75  | SE Europe                | $\Delta\text{T}$           | 8370/7820                   | Davis et al. 2003              |
| 9  | Sharkey, MN         | Charcoal                   | 3970                   | Camill et al. 2003             | 76  | Kola                     | $\delta^{18}\text{O}$      | 8180/3550                   | Jones et al. 2004              |
| 10 | NC America          | $\delta^{18}\text{O}$      | 7470/6530/4670         | Denniston et al. 1999          | 77  | Lk Victoria              | Diatoms                    | 9150/8350/7740<br>7370/7290 | Stager et al. 2003             |
| 11 | Cold Water Cv, IA   | $\delta^{18}\text{O}$      | 6730/3550<br>3290/3020 | Dorale et al. 1992             | 78  | Lk Malawi                | Si                         | 9300                        | Johnson et al. 2002            |
| 12 | Guatemala           | $\delta^{18}\text{O}$ (Cy) | 7040/3560              | Curtis et al. 1998             | 79  | Lk Malawi                | MAR                        | none                        | Johnson et al. 2002            |
| 13 | Guatemala           | $\delta^{18}\text{O}$ (Co) | 8950/4520              | Curtis et al. 1998             | 81  | Soreq Cv, Israel         | $\delta^{18}\text{O}$      | 7170/4450                   | Bar-Matthews et al. 1999       |
| 14 | Guatemala           | $\delta^{18}\text{O}$ (Py) | 9010/3250              | Curtis et al. 1998             | 82  | Red Sea                  | $\delta^{18}\text{O}$      | 9090/3730                   | Seeberg-Elverfeldt et al. 2004 |
| 15 | E Pacific           | $\delta^{18}\text{O}$      | none                   | Rosenthal 2003                 | 83  | Lk Sim, Kenia            | $\delta^{18}\text{O}$      | 8530/5590/4980              | Barker et al. 2001             |
| 16 | Yucatan             | $\delta^{18}\text{O}$ (Ph) | none                   | Hodell et al. 1995             | 84  | Lk Hall, Kenia           | $\delta^{18}\text{O}$      | 5250/4730                   | Barker et al. 2001             |
| 17 | Yucatan             | $\delta^{18}\text{O}$ (Py) | none                   | Hodell et al. 1995             | 85  | Kilimanjaro              | $\delta^{18}\text{O}$      | 4110                        | Thompson et al. 2002           |
| 18 | Costa Rica          | $\delta^{18}\text{O}$      | 7760/3890<br>7350/6680 | Lachniet et al. 2004           | 86  | Lk Abhe, Ethiopia        | Level                      | 8870/6800                   | Gasse 2000                     |
| 19 | E Canada            | Charcoal                   | 6220/4250              | Carcaillet et al. 2001         | 87  | Somalia                  | $\delta^{18}\text{O}$      | 8890/8100<br>7340/6900      | Jung et al. 2004               |
| 20 | Ecuador             | ENSO                       | 9400/3790              | Moy et al. 2002                | 88  | Qunf Cv, Oman            | $\delta^{18}\text{O}$      | none                        | Fleitmann et al. 2007          |
| 21 | E Canada            | Charcoal                   | 6550/3690              | Carcaillet et al. 2001         | 89  | Oman                     | $\delta^{18}\text{O}$      | 6940/5220/4370              | Fleitmann et al. 2003          |
| 22 | Ecuador             | GSD                        | none                   | Rodbell et al. 1999            | 90  | Arabian Sea              | $\delta^{18}\text{O}$      | 8970/7730                   | Gupta et al. 2003              |
| 23 | Huascaran, Peru     | $\delta^{18}\text{O}$      | none                   | Thompson et al. 2003           | 91  | Arabian Sea              | SSTW                       | none                        | Schulz 1995                    |
| 24 | Chile               | $\delta^{18}\text{O}$      | 6640/5920/5740         | Lamy et al. 2002               | 92  | NE Arabian Sea           | $\delta^{18}\text{O}$      | none                        | Doose-Rolinski et al. 2001     |
| 25 | Chilean Coast       | SST                        | 6700/4380              | Lamy and Hebbeln 2001          | 93  | NW Siberia               | T7                         | none                        | Hantemirov and Shiyatov 2002   |
| 26 | Haiti               | $\delta^{18}\text{O}$      | 9250/8940<br>8770/7600 | Higuera-Gundy et al. 1999      | 94  | E Arabian Sea            | $\delta^{18}\text{O}$      | 8740/4720                   | Sarkar et al. 2000             |
| 27 | New England         | Storms                     | none                   | Noren et al. 2002              | 95  | Lk Issyk-Kul, Kyrgyzstan | $\delta^{18}\text{O}$      | 8360/7950/7670              | Ricketts et al. 2001           |
| 28 | Lk Titikaka         | Level                      | none                   | Abbott et al. 1997             | 96  | Tibet                    | $\delta^{18}\text{O}$      | none                        | Fontes et al. 1996             |
| 29 | Sajama, Bolivia     | Particles                  | 4500/3500              | Thompson et al. 2003           | 97  | Dunde, China             | $\delta^{18}\text{O}$      | 7500/6970/6810<br>6260/5770 | Jung et al. 2004               |
| 30 | Sajama, Bolivia     | $\delta^{18}\text{O}$      | 4100                   | Thompson et al. 2003           | 98  | Komsomolskaia            | $\delta^2\text{H}$         | 6860/6460                   | Masson 2000                    |
| 31 | Venezuela           | $\delta^{18}\text{O}$      | 7400/6570<br>5860/4250 | Curtis et al. 1999             | 99  | N Siberia                | Pollen                     | 3490                        | Andreev et al. 2003            |
| 32 | NE Canada           | GSD                        | 7980/3250/6380         | Barber et al. 2002             | 100 | NW China                 | P (AC)                     | 8050                        | Herzschuh et al. 2004          |
| 33 | W Antarctic         | Inclination                | 7560/3090              | Brachfeld et al. 2000          | 101 | NW China                 | P (Ef)                     | 7460/6210                   | Herzschuh et al. 2004          |
| 34 | Cariaco Basin       | GSD                        | 7180                   | Haug et al. 2001               | 102 | Dongge Cv, China         | $\delta^{18}\text{O}$      | 7830/5190                   | Wang et al. 2005               |
| 35 | Cariaco Basin       | Titanium                   | none                   | Haug et al. 2001               | 103 | Vostok, Antarctica       | $\delta^2\text{H}$         | 7080                        | Petit et al. 1999              |
| 36 | Cariaco Basin       | SST                        | 8750                   | Lea et al. 2003                | 104 | N China                  | Clay                       | 8980/3760                   | Xiao et al. 2002               |
| 37 | Bermuda Rise        | $\delta^{18}\text{O}$      | 8830/3950              | Keigwin 1996                   | 105 | S China                  | Moisture                   | 9240                        | Liu et al. 2000                |
| 38 | Botuvera Cv, Brasil | $\delta^{18}\text{O}$      | 7920                   | Cruz Jr et al. 2005            | 106 | Xiangshui Cv, China      | $\delta^{18}\text{O}$      | 4960                        | Zhang et al. 2004              |
| 39 | Greenland Ice       | $\text{Be}^{10}$           | 9150/4460/4260         | Finkel and Nishiizumi 1997     | 107 | S China Sea              | $\delta^{18}\text{O}$      | 9490                        | Kienast et al. 2001            |
| 40 | Greenland Ice       | $\delta^{18}\text{O}$      | 8740/7110              | Grootes and Stuiver 1997       | 108 | N China                  | GSD                        | 8990/3980/7350              | Jin et al. 2004                |
| 41 | Greenland Ice       | SSN                        | 8320                   | Solanki et al. 2004            | 109 | S China Sea              | $\delta^{18}\text{O}$      | 8450                        | Wang et al. 1999               |
| 42 | Greenland Ice       | $\delta^{14}\text{C}$      | none                   | Stuiver et al. 1998            | 110 | Taiwan                   | LOI                        | 5200/3950                   | Huang et al. 1997              |
| 43 | W Atlantic          | $\delta^{18}\text{O}$ (Tu) | 7800/4760              | Arz and Gerhardt 2001          | 111 | S China Sea              | SSS                        | 8340/7440/7260<br>7110/5750 | Jung et al. 2004               |
| 44 | W Atlantic          | $\delta^{18}\text{O}$      | 9450/6180/5220         | Arz and Gerhardt 2001          | 112 | S China Sea              | $\delta^{18}\text{O}$      | 8600/5380                   | Wang et al. 1999               |
| 45 | Eq Atlantic         | $\Delta\text{SST}$         | none                   | Kim and Schneider 2003         | 113 | S China Sea              | Silt                       | 4740/3320/3070              | Wang et al. 1999               |
| 46 | N Atlantic          | HSG                        | 3830                   | Gupta et al. 2003              | 114 | S China Sea              | $\delta^{18}\text{O}$      | 7630/7460/5930              | Wang et al. 1999               |
| 47 | N Atlantic          | LG                         | 4750                   | Bond 1997                      | 115 | Dongge Cv, China         | $\delta^{18}\text{O}$      | none                        | Yuan et al. 2004               |
| 48 | Trop Atlantic       | $\delta^{18}\text{O}$      | 6550                   | Knaack 1997                    | 116 | Sulu Sea                 | $\delta^{18}\text{O}$      | 3240/7730                   | Rosenthal 2003                 |
| 49 | Trop Atlantic       | SST                        | none                   | DeMenocal et al. 2000          | 117 | W Pacific                | $\delta^{18}\text{O}$ (81) | none                        | Stott et al. 2004              |
| 50 | N Atlantic          | HSG                        | 4100                   | Bond et al. 2001               | 118 | E China Sea              | SST                        | 9370                        | Sun et al. 2005                |
| 51 | Canary              | $\delta^{18}\text{O}$      | none                   | Freudenthal et al. 2002        | 119 | E China Sea              | SST                        | none                        | Fengming et al. 2008           |
| 52 | Ireland             | $\delta^{18}\text{O}$      | 8960/8140              | McDermott 2004                 | 120 | W Pacific                | $\delta^{18}\text{O}$      | none                        | Rosenthal 2003                 |
| 53 | NW Morocco          | $\delta^{18}\text{O}$      | 7850/3930/4080         | Hodell et al. 2001a            | 121 | W Pacific                | $\delta^{18}\text{O}$ (76) | 8420/7270                   | Stott et al. 2004              |
| 54 | SW Europe           | $\Delta\text{T}$           | 8970/3320              | Davis et al. 2003              | 122 | NW Pacific               | %Nitzschia                 | 6290/4880                   | Shimada et al. 2004            |
| 55 | NW Europe           | $\Delta\text{T}$           | none                   | Davis et al. 2003              | 123 | NW Pacific               | %Ozeanica                  | 6170                        | Shimada et al. 2004            |
| 56 | S Atlantic          | LG                         | 8760/3820/3190         | Hodell et al. 2001b            | 124 | S Australia              | T                          | none                        | Cook and Buckley 2000          |
| 57 | Swiss Alps          | T7                         | 7950/6030              | Wick et al. 2003               | 125 | Tasmania                 | T                          | none                        | Cook and Buckley 2000          |
| 58 | Swiss Alps          | P                          | 7920                   | Wick et al. 2003               | 126 | SW Australia             | Particles                  | 8410/8310                   | Stanley and Deckker 2002       |
| 59 | Swiss Alps          | P                          | 7920/5980              | Wick et al. 2003               | 127 | Taylor dome              | $\delta^{18}\text{O}$      | 3750                        | Grootes et al. 2001            |
| 60 | C Italy             | Mg/Ca T                    | 5950/3270              | Drysdale et al. 2006           | 128 | Taylor dome              | $\delta^2\text{H}$         | none                        | Steig et al. 1998              |
| 61 | Angola Basin        | $\text{U}_{37}^k$ SST      | none                   | Kim and Schneider 2003         | 129 | Lk Ioannina, Greece      | $\delta^{18}\text{O}$      | 4050                        | Frogley and Griffiths 2001     |
| 62 | C Italy             | $\delta^{18}\text{O}$      | 5950                   | Drysdale et al. 2006           | 131 | Lk Akgöl, Turkey         | $\delta^{18}\text{O}$      | none                        | Roberts et al. 2008            |
| 63 | S Germany           | $\delta^{18}\text{O}$      | 8130/8050/7190         | von Grafenstein et al. 1998    | 132 | Lk Acigöl, Turkey        | $\delta^{18}\text{O}$      | 3160                        | Roberts et al. 2011            |
| 64 | Sahel               | $\delta^{18}\text{O}$      | 9070/6190              | Gasse 2002                     | 133 | Lk Frassino, Italy       | $\delta^{18}\text{O}$      | none                        | Roberts et al. 2008            |
| 65 | N Atlantic          | SST                        | 7430/4820              | Sarnthein et al. 2003          | 134 | Lk Gölhisar, Turkey      | $\delta^{18}\text{O}$      | 3070                        | Roberts et al. 2011            |
| 66 | N Norway            | T                          | 6940                   | Husum and Hald 2004            | 135 | Lk Pergusa, Italy        | $\delta^{18}\text{O}$      | 6620                        | Roberts et al. 2008            |
| 67 | Sweden              | GSD                        | 9180/8350<br>7700/3760 | Rubensdotter and Rosqvist 2003 |     |                          |                            |                             |                                |

## References

- Abbott, M. B., Binford, M. W., Brenner, M., Curtis, J. H., Kelts, K. R., 1997. A 3500  $^{14}\text{C}$  yr high-resolution sediment record of lake level changes in Lake Titicaca, Bolivia/Peru. *Quaternary Research* 47 (2), 169–180.
- Andreev, A. A., Tarasov, P. E., Siebert, C., Ebel, T., Klimanov, V. A., Melles, M., Bobrov, A. A., Dereviagin, A. Y., Lubinski, D. J., Hubberten, H.-W., 2003. Late Pleistocene and Holocene vegetation and climate on the northern Taymyr Peninsula, Arctic Russia. *Boreas* 32 (3), 484–505.
- Arz, H. W., Gerhardt, S., 2001. Millennial-scale changes of surface- and deep-water flow in the western tropical Atlantic linked to Northern Hemisphere high-latitude climate during the Holocene. *Geology* 29 (3), 239–242.
- Bahr, A., Lamy, F., Arz, H. W., Kuhlmann, H., Wefer, G., 2005. Late glacial to Holocene climate and sedimentation history in the NW Black Sea. *Marine Geology* 214 (4), 309–322.
- Bar-Matthews, M., Ayalon, A., Kaufman, A., Wasserburg, G. J., 1999. The Eastern Mediterranean paleoclimate as a reflection of regional events: Soreq cave, Israel. *Earth and Planetary Science Letters* 166 (1–2), 85–95.
- Barber, D. C., Dyke, A., Hilaire-Marcel, C., Jennings, A. E., Andrews, J. T., Kerwin, M. W., Bilodeau, G., McNeely, R., Soutn, J., Morehead, M. D., Gagnon, J.-M., 2002. Forcing of the cold event of 8,200 years ago by catastrophic drainage of Laurentide lakes. *Nature* 400 (6742), 344–348.
- Barker, P. A., Street-Perrott, F. A., Leng, M. J., Greenwood, P. B., Swain, D. L., Perrott, R. A., Telford, R. J., Ficken, K. J., 2001. A 14,000-Year Oxygen Isotope Record from Diatom Silica in Two Alpine Lakes on Mt. Kenya. *Science* 292 (5525), 2307–2310.
- Begon, M., Harper, J. L., Townsend, C. R., 1993. *Ecology: Individual, Populations and Communities*, 2nd Edition. Blackwell Scientific Publications, Oxford.
- Benson, L., Kashgarian, M., Rye, R., Lund, S., Paillet, F., Smoot, J., Kester, C., Mensing, S., Meko, D., 2002. Holocene multidecadal and multicentennial droughts affecting Northern California and Nevada. *Quaternary Science Reviews* 21 (4–6), 659–682.
- Bloom, D. E., Sachs, J. D., Collier, P., Udry, C., 1998. Geography, demography and economic growth in Africa. *Brookings Papers on Economic Activity* 1998 (2), 207–295.
- Bond, G., 1997. A Pervasive Millennial-Scale Cycle in North Atlantic Holocene and Glacial Climates. *Science* 278 (5341), 1257–1266.
- Bond, G., Kromer, B., Beer, J., 2001. Persistent solar influence on North Atlantic climate during the Holocene. *Science* 294 (5549), 2130–2136.
- Bonnefille, R., Chalié, F., 2000. Pollen-inferred precipitation time-series from equatorial mountains, Africa, the last 40 kyr BP. *Global and Planetary Change* 26 (1–3), 25–50.
- Brachfeld, S., Acton, G. D., Guyodo, Y., Banerjee, S. K., 2000. High-resolution paleomagnetic records from Holocene sediments from the Palmer Deep, Western Antarctic Peninsula. *Earth and Planetary Science Letters* 181 (3), 429–441.
- Braidwood, L., Braidwood, R. J., 1949. On the treatment of the prehistoric Near Eastern materials in Steward's "Cultural Causality and Law". *American Anthropologist* 51 (4), 665–669.
- Camill, P., Umbanhowar Jr, C. E., Teed, R., Geiss, C. E., Aldinger, J., Dvorak, L., Kenning, J., Limmer, J., Walkup, K., 2003. Late-glacial and Holocene climatic effects on fire and vegetation dynamics at the prairie forest ecotone in south-central Minnesota. *Journal of Ecology* 91 (5), 822–836.
- Carcaillet, C., Bergeron, Y., Richard, P. J. H., Fréchette, B., Gauthier, S., Prairie, Y. T., 2001. Change of fire frequency in the eastern Canadian boreal forests during the Holocene: does vegetation composition or climate trigger the fire regime? *Journal of Ecology* 89 (6), 930–946.
- Chapman, M., Shackleton, N., 2000. Evidence of 550-year and 1000-year cyclicities in North Atlantic circulation patterns during the Holocene. *The Holocene* 10 (3), 287–291.
- Claussen, M., Brovkin, V., 1999. A new model for climate system analysis: Outline of the model and application to palaeoclimate simulations. *Environmental Modeling and Assessment* 4 (4), 209–216.
- Cook, E., Buckley, B., 2000. Warm-season temperatures since 1600 BC reconstructed from Tasmanian tree rings and their relationship to large-scale sea surface temperature anomalies. *Climate Dynamics* 16 (2–3), 79–91.
- Cruz Jr, F. W., Burns, S. J., Karmann, I., Sharp, W. D., Vuille, M., Cardoso, A. O., Ferrari, J. A., Dias, P. L. S., Viana Jr., O., 2005. Insolation-driven changes in atmospheric circulation over the past 116,000 years in subtropical Brazil. *Nature* 434 (7029), 63–66.
- Curtis, J. H., Brenner, M., Hodel, D. A., 1999. Climate change in the Lake Valencia Basin, Venezuela, ~12600 yr BP to present. *The Holocene* 9 (5), 609–619.
- Curtis, J. H., Brenner, M., Hodel, D. A., Balser, R. A., Islebe, G. A., Hooghiemstra, H., 1998. A multi-proxy study of Holocene environmental change in Lowlands of Peten, Guatemala. *Journal of Paleolimnology* 19 (2), 139–159.
- Davis, B. A. S., Brewer, S., Stevenson, A. C., Guiot, J., 2003. The temperature of Europe during the Holocene reconstructed from pollen data. *Quaternary Science Reviews* 22 (15–17), 1701–1716.
- Davis, O. K., 1992. Rapid Climate Change in Coastal Southern California Inferred from Pollen analysis of San Joaquin Marsh. *Quaternary Research* 23 (1), 227–235.
- DeMenocal, P. B., Ortiz, J., Guilderson, T., Adkins, J., Sarnthein, M., Baker, L., Yarusinsky, M., 2000. Abrupt onset and termination of the African Humid Period: rapid climate responses to gradual insolation forcing. *Quaternary science reviews* 19 (1–5), 347–361.
- Denniston, R. F., Gonzalez, L. A., Baker, R. G., Reagan, M. K., Asmerom, Y., Edwards, R. L., Alexander, E. C., 1999. Speleothem evidence for Holocene fluctuations of the prairie-forest ecotone, north-central USA. *The Holocene* 9 (6), 671–676.
- Doose-Rolinski, H., Rogalla, U., Scheeder, G., 2001. High resolution temperature and evaporation changes during the late Holocene in the northeastern Arabian Sea. *Paleoceanography* 16 (4), 358–367.
- Dorale, J. A., Gonzalez, L. A., Reagan, M. K., Pickett, D. A., Murrell, M. T., Baker, R. G., 1992. A High-Resolution Record of Holocene Climate Change in Speleothem Calcite from Cold Water Cave, Northeast Iowa. *Science* 258 (5088), 1626–1630.
- Drysdale, R., Zanchetta, G., Hellstrom, J., Maas, R., Fallick, A., Pickett, M., Cartwright, I., Piccini, L., 2006. Late Holocene drought responsible for the collapse of Old World civilizations is recorded in an Italian cave flowstone. *Geology* 34 (2), 101–104.
- Ehrlich, P. R., Holdren, J. P., 1971. Impact of population growth. *Science* 171 (977), 1212–1217.
- Fengming, C., Tiegang, L., Lihua, Z., Jun, Y., 2008. A Holocene paleotemperature record based on radiolaria from the northern Okinawa Trough (East China Sea). *Quaternary International* 183 (1), 115–122.
- Finkel, R. C., Nishiizumi, K., 1997. Beryllium 10 concentrations in the Greenland Ice Sheet Project 2 ice core from 340 ka. *Journal of Geophysical Research* 102 (C12), 26699–26706.
- Fisher, R. A., 1930. *The Genetical Theory of Natural Selection*. Dover, New York.
- Fleitmann, D., Burns, S. J., Mangini, A., Mudelsee, M., Kramers, J., Villa, I., Neff, U., Al-Subbary, A. A., Buettner, A., Hippler, D., Matter, A., Sij, B., Aa, A.-s., 2007. Holocene ITCZ and Indian monsoon dynamics recorded in stalagmites from Oman and Yemen (Socotra). *Quaternary Science Reviews* 26 (1–2), 170–188.
- Fleitmann, D., Burns, S. J., Mudelsee, M., Neff, U., Kramers, J., Mangini, A., Matter, A., 2003. Holocene Forcing of the Indian Monsoon Recorded in a Stalagmite from Southern Oman. *Science* 300 (5626), 1737–1739.
- Fontes, J.-C., Gasse, F., Gibert, E., 1996. Holocene environmental changes in Lake Bangong basin (Western Tibet). Part 1: Chronology and stable isotopes of carbonates of a Holocene lacustrine core. *Palaeogeography, Palaeoclimatology, Palaeoecology* 120 (1–2), 25–47.
- Freudenthal, T., Meggers, H., Henderiks, J., 2002. Upwelling intensity and filament activity off Morocco during the last 250,000 years. *Deep Sea Research Part II: Topical Studies in Oceanography*

- graphy 49 (17), 3655–3674.
- Frogley, M., Griffiths, H., 2001. Historical biogeography and Late Quaternary environmental change of Lake Pamvotis, Ioannina (northwestern Greece): evidence from ostracods. *Journal of Biogeography* 28 (6), 745–756.
- Gallup, J. L., Sachs, J. D., 2000. Agriculture, Climate, and Technology: Why Are the Tropics Falling Behind? *American Journal of Agricultural Economics* 82, 731–737.
- Gasse, F., 2000. Hydrological changes in the African tropics since the Last Glacial Maximum. *Quaternary Science Reviews* 19 (1), 189–211.
- Gasse, F., 2002. Diatom-inferred salinity and carbonate oxygen isotopes in Holocene waterbodies of the western Sahara and Sahel (Africa). *Quaternary science reviews* 21 (7), 737–767.
- Gaston, K. J., 2000. Global patterns in biodiversity. *Nature* 405 (6783), 220–227.
- Grootes, P. M., Steig, E. J., Stuiver, M., Waddington, E. D., Morse, D. L., Land, S. V., 2001. The Taylor Dome Antarctic  $^{18}\text{O}$  Record and Globally Synchronous Changes in Climate. *Quaternary Research* 298 (3), 289–298.
- Grootes, P. M., Stuiver, M., 1997. Oxygen 18/16 variability in Greenland snow and ice with  $10^{-3}$ - to  $10^5$ -year time resolution. *Journal of Geophysical Research* 102 (C12), 26455–26470.
- Gupta, A. K., Anderson, D. M., Overpeck, J. T., 2003. Abrupt changes in the Asian southwest monsoon during the Holocene and their links to the North Atlantic Ocean. *Nature* 421 (6921), 4–7.
- Hantemirov, R. M., Shiyatov, S. G., 2002. A continuous multimillennial ring-width chronology in Yamal, northwestern Siberia. *The Holocene* 12 (6), 717–726.
- Haug, G. H., Hughen, K. A., Sigman, D. M., Peterson, L. C., Röhl, U., 2001. Southward migration of the intertropical convergence zone through the Holocene. *Science* 293 (5533), 1304–1308.
- Herzschuh, U., Tarasov, P. E., Wu, B., Hartmann, K., 2004. Holocene vegetation and climate of the Alashan Plateau, NW China, reconstructed from pollen data. *Palaeogeography, Palaeoclimatology, Palaeoecology* 211 (1–2), 1–17.
- Higuera-Gundy, A., Brenner, M., Hodell, D. A., Curtis, J. H., Leyden, B. W., Binford, M. W., Florida, I., 1999. A 10,300  $^{14}\text{C}$  yr Record of Climate and Vegetation Change from Haiti. *Quaternary Research* 170 (2), 159–170.
- Hodell, D. A., Curtis, J. H., Brenner, M., 1995. Possible role of climate in the collapse of the Classic Maya Civilization. *Nature* 375 (6530), 391–394.
- Hodell, D. A., Curtis, J. H., Sierro, F. J., Raymo, M. E., 2001a. Correlation of late Miocene to early Pliocene sequences between the Mediterranean and North Atlantic. *Paleoceanography* 16 (2), 164–178.
- Hodell, D. A., Kanfoush, S., Shemesh, A., Crosta, X., 2001b. Abrupt cooling of Antarctic surface waters and sea ice expansion in the South Atlantic sector of the Southern Ocean at 5000 cal yr BP. *Quaternary International* 198 (2), 191–198.
- Holmgren, K., Lee-Thorp, J. A., Cooper, G. R. J., Lundblad, K., Partridge, T. C., Scott, L., Sithaldeen, R., Siep Talma, A., Tyson, P. D., 2003. Persistent millennial-scale climatic variability over the past 25,000 years in Southern Africa. *Quaternary Science Reviews* 22 (21–22), 2311–2326.
- Hu, F. S., Ito, E., Brubaker, L. B., Anderson, P. M., 1998. Ostracode Geochemical Record of Holocene Climatic Change and Implications for Vegetational Response in the Northwestern Alaska Range. *Quaternary Research* 95 (49), 86–95.
- Huang, C., Liew, P., Zhao, M., 1997. Deep sea and lake records of the Southeast Asian paleomonsoons for the last 25 thousand years. *Earth and Planetary Science Letters* 146 (1–2), 59–72.
- Hughes, M. K., Graumlich, L. J., 1996. Climatic variations and forcing mechanisms of the last 2000 years. Multi-millennial dendroclimatic studies from the western United States. *NATO ASI Series Global Environmental Change* 41, 109–124.
- Husum, K., Hald, M., 2004. A continuous marine record 8000–1600 cal. yr BP from the Malangenfjord, north Norway: foraminiferal and isotopic evidence. *The Holocene* 14 (6), 877–887.
- Jin, Z., Wu, J., Cao, J., Wang, S., Shen, J., 2004. Holocene chemical weathering and climatic oscillations in north China: evidence from lacustrine sediments. *Boreas* 33 (3), 260–266.
- Johnson, T. C., Brown, E. T., Mcmanus, J., Barry, S., 2002. A High-Resolution Paleoclimate Record Spanning the Past 25,000 Years in Southern East Africa. *Science* 296 (5565), 3–6.
- Jones, V., Leng, M. J., Solovieva, N., Sloane, H., Tarasov, P. E., 2004. Holocene climate of the Kola Peninsula; evidence from the oxygen isotope record of diatom silica. *Quaternary Science Reviews* 23 (7–8), 833–839.
- Jung, S. J. A., Davies, G. R., Ganssen, G. M., Kroon, D., 2004. Synchronous Holocene sea surface temperature and rainfall variations in the Asian monsoon system. *Quaternary Science Reviews* 23 (20–22), 2207–2218.
- Keigwin, L. D., 1996. The little Ice Age and medieval warm period in the Sargasso Sea. *Science* 274 (5292), 1503–1508.
- Kienast, M., Calvert, S. E., Pelejero, C., Grimalt, J. O., 2001. A critical review of marine sedimentary  $\delta^{13}\text{C}$  org-pCO<sub>2</sub> estimates: New palaeorecords from the South China Sea and a revisit of other low-latitude  $\delta^{13}\text{C}$  org-pCO<sub>2</sub> records. *Global Biogeochemical Cycles* 15 (1), 113–127.
- Kim, J.-H., Schneider, R. R., 2003. Low-latitude control of inter-hemispheric sea-surface temperature contrast in the tropical Atlantic over the past 21 kyears: the possible role of SE trade winds. *Climate Dynamics* 21 (3–4), 337–347.
- Kisdi, E., Geritz, S. A. H., 2010. Adaptive dynamics: a framework to model evolution in the ecological theatre. *Journal of Mathematical Biology* 61 (1), 165–9.
- Knaack, J. J., 1997. Eine neue Transferfunktion zur Rekonstruktion der Paläoproduktivität aus Gemeinschaften mariner Diatomeen. *Berichte des Geologisch-Paläontologischen Instituts der Universität zu Kiel* 83, 1–118.
- Lachniet, M. S., Asmerom, Y., Burns, S. J., Patterson, W. P., Polyak, V. J., Seltzer, G. O., 2004. Tropical response to the 8200 yr B.P. cold event? Speleothem isotopes indicate a weakened early Holocene monsoon in Costa Rica. *Geology* 32 (11), 957–960.
- Laird, K. R., Fritz, S. C., Maasch, K. A., Cumming, B. F., 1996. Greater drought intensity and frequency before A.D. ~1200 in the northern Great Plains, USA. *Nature* 384 (6609), 552–554.
- Lamy, F., Hebbeln, D., 2001. Holocene rainfall variability in southern Chile: a marine record of latitudinal shifts of the Southern Westerlies. *Earth and Planetary Science Letters* 185 (3–4), 369–382.
- Lamy, F., Ru, C., Hebbeln, D., Wefer, G., America, S., 2002. High- and low-latitude climate control on the position of the southern Peru-Chile Current during the Holocene. *October 17 (1028)*, 10.
- Lea, D. W., Pak, D. K., Peterson, L. C., Hughen, K. A., 2003. Synchronicity of tropical and high-latitude Atlantic temperatures over the last glacial termination. *Science* 301 (5638), 1361–1364.
- Leemans, R., Cramer, W. P., 1991. The IIASA database for mean monthly values of temperature, precipitation and cloudiness of a global terrestrial grid. Research report, International Institute of Applied Systems Analyses, Laxenburg.
- Lemmen, C., 2010. World distribution of land cover changes during Pre- and Protohistoric Times and estimation of induced carbon releases. *Géomorphologie : relief, processus, environnement* 4 (2009), 303–312.
- Lemmen, C., Wirtz, K. W., 2010. Socio-technological revolutions and migration waves: re-examining early world history with a numerical model. In: Gronenborn, D., Petrasch, J. (Eds.), *The Spread of the Neolithic to Central Europe*. Vol. 4, I of RGZM Tagungen. Verlag des Römisch-Germanischen Zentralmuseums, Mainz, pp. 25–38.
- Lieth, H., 1975. Modeling the primary productivity of the world. *Primary Productivity of the Biosphere* 14, 237–263.
- Liu, J., Houyuan, L., Negendank, J., Mingram, J., Xiangjun, L., Wenyan, W., Guoqiang, C., 2000. Periodicity of Holocene climatic variations in the Huguangyan Maar Lake. *Chinese Science Bulletin* 45 (18), 1712–1718.
- Masson, V., 2000. Holocene Climate Variability in Antarctica Based on 11 Ice-Core Isotopic Records. *Quaternary Research* 54 (3), 348–358.

- McDermott, F., 2004. Palaeo-climate reconstruction from stable isotope variations in speleothems: a review. *Quaternary Science Reviews* 23 (7-8), 901–918.
- Moy, C. M., Seltzer, G. O., Rodbell, D. T., Anderson, D. M., 2002. Variability of El Niño/Southern Oscillation activity at millennial timescales during the Holocene epoch. *Nature* 420 (6912), 162–165.
- Noren, A. J., Bierman, P. R., Lini, A., 2002. Millennial-scale storminess variability in the northeastern United States during the Holocene epoch. *Nature* 419 (6909), 821–824.
- Oba, T., Murayama, M., 2004. Sea-surface temperature and salinity changes in the northwest Pacific since the Last Glacial Maximum. *Journal of Quaternary Science* 19 (4), 335–346.
- Petit, J. R., Raynaud, D., Basile, I., Chappellaz, J., Davisk, M., Ritz, C., Delmotte, M., Legrand, M., Lorius, C., Pe, L., Saltzman, E., 1999. Climate and atmospheric history of the past 420,000 years from the Vostok ice core, Antarctica. *Nature* 399 (6735), 429–436.
- Renfrew, C., Level, E. V., 1979. Exploring dominance: predicting politics from centers. In: Renfrew, C., Cooke, K. (Eds.), *Transformations: Mathematical Approaches to Culture Change*. Academic Press, New York, pp. 145–166.
- Ricketts, R. D., Johnson, T. C., Brown, E. T., Rasmussen, K. A., Romanovsky, V. V., 2001. The Holocene paleolimnology of Lake Issyk-Kul, Kyrgyzstan: trace element and stable isotope composition of ostracodes. *Palaeogeography, Palaeoclimatology, Palaeoecology* 176 (1-4), 207–227.
- Roberts, N., Eastwood, W. J., Kuzucuoglu, C., Fiorentino, G., Caracuta, V., 2011. Climatic, vegetation and cultural change in the eastern Mediterranean during the mid-Holocene environmental transition. *The Holocene* 21 (1), 147–162.
- Roberts, N., Jones, M., Benkaddour, A., Eastwood, W. J., Filippi, M., Frogley, M., Lamb, H., Leng, M. J., Reed, J., Stein, M., Stevens, L., Valero-Garcés, B., Zanchetta, G., 2008. Stable isotope records of Late Quaternary climate and hydrology from Mediterranean lakes: the ISOMED synthesis. *Quaternary Science Reviews* 27 (25-26), 2426–2441.
- Rodbell, D. T., Seltzer, G. O., Anderson, D. M., Abbott, M. B., Enfield, D. B., Newman, J. H., 1999. An ~15,000-Year Record of El-Niño Alluviation in Southwestern Ecuador. *Science* 283 (5401), 516–520.
- Rosenthal, Y., 2003. The amplitude and phasing of climate change during the last deglaciation in the Sulu Sea, western equatorial Pacific. *Geophysical Research Letters* 30 (8), 1–4.
- Rubensdotter, L., Rosqvist, G., 2003. The effect of geomorphological setting on Holocene lake sediment variability, northern Swedish Lapland. *Journal of Quaternary Science* 18 (8), 757–767.
- Sarkar, A., Ramesh, R., Somayajulu, B. L. K., Agnihotri, R., 2000. High resolution Holocene monsoon record from the eastern Arabian Sea. *Earth and Planetary Science Letters* 177 (3-4), 2000–2000.
- Sarnthein, M., van Kreveld, S., Erlenkeuser, H., Grootes, P. M., Kucera, M., Pflaumann, U., Schulz, M., 2003. Centennial-to-millennial-scale periodicities of Holocene climate and sediment injections off the western Barents shelf, 75° N. *Boreas* 32 (3), 447–461.
- Schulz, H., 1995. Meeresoberflächentemperaturen vor 10000 Jahren – Auswirkungen des frühholozänen Insulationsmaximums. *Tech. rep.*
- Seeberg-Elverfeldt, I., Lange, C. B., Arz, H. W., Pätzold, J., Pike, J., 2004. The significance of diatoms in the formation of laminated sediments of the Shaban Deep, Northern Red Sea. *Marine Geology* 209 (1-4), 279–301.
- Shimada, C., Ikehara, K., Tanimura, Y., Hasegawa, S., 2004. Millennial-scale variability of Holocene hydrography in the south-western Okhotsk Sea: diatom evidence. *The Holocene* 14 (5), 641–650.
- Solanki, S. K., Usoskin, I. G., Kromer, B., Schüssler, M., Beer, J., 2004. Unusual activity of the Sun during recent decades compared to the previous 11,000 years. *Nature* 431 (7012), 1084.
- Sperling, M., Schmiedl, G., Emeis, K. C., Erlenkeuser, H., Grootes, P. M., 2003. Black Sea impact on the formation of eastern Mediterranean sapropel S1? Evidence from the Marmara Sea. *Palaeogeography, Palaeoclimatology, Palaeoecology* 190 (1), 9–21.
- Stager, J. C., Cumming, B. F., Meeker, L. D., 2003. A 10,000-year high-resolution diatom record from Pilkington Bay, Lake Victoria, East Africa. *Quaternary Research* 59 (2), 172–181.
- Stanley, S., Deckker, P. D., 2002. A Holocene record of allochthonous, aeolian mineral grains in an Australian alpine lake; implications for the history of climate change in southeastern Australia. *Journal of Paleolimnology* 27 (2), 207–219.
- Steig, E. J., Brook, E. J., White, J. W. C., Sucher, C. M., Bender, M. L., Lehman, S. J., Morse, D. L., Waddington, E. D., Clow, G. D., 1998. Synchronous Climate Changes in Antarctica and the North Atlantic. *Science* 282 (5386), 92.
- Stott, L. D., Cannariato, K. G., Thunell, R., Haug, G. H., Koutavas, A., Lund, S., 2004. Decline of surface temperature and salinity in the western tropical Pacific Ocean in the Holocene epoch. *Nature* 431 (7004), 56–59.
- Stuiver, M., Reimer, P. J., Bard, E., Beck, J. W., Burr, G. S., Hughen, K. A., Kromer, B., McCormac, G., van der Plicht, J., Spurk, M., 1998. INTCAL98 radiocarbon age calibration, 24,000–0 cal BP. *Radiocarbon* 40 (3), 1041–1083.
- Sun, D., Gagan, M. K., Cheng, H., Scott-Gagan, H., Dykoski, C. A., Edwards, R. L., Su, R., 2005. Seasonal and interannual variability of the Mid-Holocene East Asian monsoon in coral delta O-18 records from the South China Sea. *Earth and planetary science letters* 237 (1-2), 69–84.
- Thompson, L. G., Mosley-thompson, E., Davis, M. E., Henderson, K. A., Brecher, H. H., Zagorodnov, V. S., Mashiotto, T. A., Lin, P.-n., Mikhalenko, V. N., Hardy, D. R., Beer, J., 2002. Kilimanjaro ice core records: Evidence of Holocene climate change in tropical Africa. *Science* 298 (5593), 589–593.
- Thompson, L. G., Mosley-Thompson, E., Davis, M. E., Lin, P.-n., Henderson, K. A., Mashiotto, T. A., 2003. Tropical glacier and ice core evidence of climate change on annual to millennial time scales. *Climatic Change* 59 (1-2), 137–155.
- von Grafenstein, U., Erlenkeuser, H., Müller, J., Jouzel, J., Johnsen, S. J., 1998. The cold event 8200 years ago documented in oxygen isotope records of precipitation in Europe and Greenland. *Climate Dynamics* 14 (2), 73–81.
- Wang, L., Sarnthein, M., Erlenkeuser, H., 1999. East Asian monsoon climate during the Late Pleistocene: high-resolution sediment records from the South China Sea. *Marine Geology* 156 (1-4), 245–284.
- Wang, Y., Cheng, H., Edwards, R., He, Y., 2005. The Holocene Asian monsoon: links to solar changes and North Atlantic climate. *Science* 308 (5723), 854–857.
- Wang, Y., van Cappellen, P., 1996. A multicomponent reactive transport model of early diagenesis: Application to redox cycling in coastal marine sediments. *Geochimica et Cosmochimica Acta* 60 (16), 2993–3014.
- Wick, L., Lemcke, G., Sturm, M., 2003. Evidence of Lateglacial and Holocene climatic change and human impact in eastern Anatolia: high-resolution pollen, charcoal, isotopic and geochemical records from the laminated sediments of Lake Van, Turkey. *The Holocene* 13 (5), 665–675.
- Wirtz, K. W., Lemmen, C., 2003. A global dynamic model for the neolithic transition. *Climatic Change* 59 (3), 333–367.
- Wirtz, K. W., Lohmann, G., Bernhardt, K., Lemmen, C., 2010. Mid-Holocene regional reorganization of climate variability: Analyses of proxy data in the frequency domain. *Palaeogeography, Palaeoclimatology, Palaeoecology* 298 (3-4), 189–200.
- Xiao, J., Nakamura, T., Lu, H., Zhang, G., 2002. Holocene climate changes over the desert/loess transition of north-central China. *Earth and Planetary Science Letters* 197 (1-2), 11–18.
- Yu, S.-y., 2003. Centennial-scale cycles in middle Holocene sea level along the southeastern Swedish Baltic coast. *GSA Bulletin* 115 (11), 1404–1409.
- Yuan, D., Cheng, H., Edwards, R., 2004. Timing, duration, and transitions of the last interglacial Asian monsoon. *Science* 304 (5670), 575.
- Zhang, M., Yuan, D., Lin, Y., Qin, J., 2004. A 6000-year high-

resolution climatic record from a stalagmite in Xiangshui Cave, Guilin, China. *The Holocene* 14 (5), 697–702.
